# Supplementary material for: A Survey on Predictive Maintenance for Industry 4.0
Source: arXiv:2002.08224 source file (2020-02-05)
Supplement: Supplementary file 1 [file Appendix.tex]

\chapter{Framework Data by Category}

	\section{Data of the Category Goals}
1=Availability; 2=Reliability; 3=Safety; 4=Productivity; 5=Spare Part Inventory Reduction; 6=Cost Minimization; 7=Minimize Downtime; 8=Prolong Machine/Component Life; 9=No Goals Mentioned

% [inline block 0: 14 envs, 83713 chars -> data_tex | \begin{longtable}{|l|p{.08cm}|p{.08cm}|p{.08cm}|p{.08cm}|p{.08cm}|p{.08cm}|p{.08cm}|p{.08cm}|p{.08cm}||l|p{.08cm}|p{.08c...]


%\ohead{\pagemark}
%\cfoot{}
%\cohead{}
%\ihead{\headmark}
%\setkomafont{pageheadfoot}{\normalfont\bfseries}
%\setkomafont{pagenumber}{\normalfont\bfseries}
%\automark{chapter}

\chapter{J48 Algorithm Decision Trees}

\begin{figure}[h]
	\centering
	\includegraphics[width=\textwidth]{figures/treeid4.png}
	\caption{J48 Decision Tree for Availability (ID 4)}
	\label{img:treeid4}
\end{figure}

\begin{figure}[h]
	\centering
	\includegraphics[width=\textwidth]{figures/treeid5.png}
	\caption{J48 Decision Tree for Reliability (ID 5)}
	\label{img:treeid4}
\end{figure}

\begin{figure}[h]
	\centering
	\includegraphics[width=\textwidth]{figures/treeid6.png}
	\caption{J48 Decision Tree for Safety (ID 6)}
	\label{img:treeid6}
\end{figure}

\begin{figure}[h]
	\centering
	\includegraphics[width=\textwidth, height=\textheight]{figures/treeid2.png}
	\caption{J48 Decision Tree for Publication Type (ID 2) }
	\label{img:treeid2}
\end{figure}

\begin{figure}[h]
	\centering
	\includegraphics[width=\textwidth, height=\textheight]{figures/treeid7.png}
	\caption{J48 Decision Tree for Productivity (ID 7)}
	\label{img:treeid7}
\end{figure}

\begin{figure}[h]
	\centering
	\includegraphics[width=\textwidth]{figures/treeid8.png}
	\caption{J48 Decision Tree for Spare Part Inventory Reduction (ID 8)}
	\label{img:treeid8}
\end{figure}

\begin{figure}[h]
	\centering
	\includegraphics[width=\textwidth]{figures/treeid9.png}
	\caption{J48 Decision Tree for Cost Minimization (ID 9)}
	\label{img:treeid9}
\end{figure}

\begin{figure}[h]
	\centering
	\includegraphics[width=\textwidth, height=\textheight]{figures/treeid10.png}
	\caption{J48 Decision Tree for Minimize Downtime (ID 10) }
	\label{img:treeid10}
\end{figure}

\begin{figure}[h]
	\centering
	\includegraphics[width=\textwidth]{figures/treeid11.png}
	\caption{J48 Decision Tree for Prolong Machine/Component Life (ID 11)}
	\label{img:treeid11}
\end{figure}

\begin{figure}[h]
	\centering
	\includegraphics[width=\textwidth]{figures/treeid12.png}
	\caption{J48 Decision Tree for No Goals Mentioned (ID 12)}
	\label{img:treeid12}
\end{figure}

\begin{figure}[h]
	\centering
	\includegraphics[width=\textwidth]{figures/treeid13.png}
	\caption{J48 Decision Tree for (Numeric) Simulation (ID 13)}
	\label{img:treeid13}
\end{figure}

\begin{figure}[h]
	\centering
	\includegraphics[width=\textwidth]{figures/treeid14.png}
	\caption{J48 Decision Tree for Experimental Evaluation (ID 14)}
	\label{img:treeid14}
\end{figure}

\begin{figure}[h]
	\centering
	\includegraphics[width=\textwidth]{figures/treeid15.png}
	\caption{J48 Decision Tree for Evaluation based on Real Data (ID 15)}
	\label{img:treeid15}
\end{figure}

\begin{figure}[h]
	\centering
	\includegraphics[width=\textwidth]{figures/treeid16.png}
	\caption{J48 Decision Tree for Comp. with convent. Maint. Policies (ID 16)}
	\label{img:treeid16}
\end{figure}

\begin{figure}[h]
	\centering
	\includegraphics[width=\textwidth]{figures/treeid19.png}
	\caption{J48 Decision Tree for Grouping Maintenance Actions (ID 19)}
	\label{img:treeid19}
\end{figure}

\begin{figure}[h]
	\centering
	\includegraphics[width=\textwidth]{figures/treeid20.png}
	\caption{J48 Decision Tree for Inspection-Based Monitoring (ID 20)}
	\label{img:treeid20}
\end{figure}

\begin{figure}[h]
	\centering
	\includegraphics[width=\textwidth, height=\textheight]{figures/treeid21.png}
	\caption{J48 Decision Tree for Sensor-Based Monitoring (ID 21) }
	\label{img:treeid21}
\end{figure}

\begin{figure}[h]
	\centering
	\includegraphics[width=\textwidth, height=\textheight]{figures/treeid22.png}
	\caption{J48 Decision Tree for Online/Real Time Monitoring (ID 22)}
	\label{img:treeid22}
\end{figure}

\begin{figure}[h]
	\centering
	\includegraphics[width=\textwidth, height=\textheight]{figures/treeid23.png}
	\caption{J48 Decision Tree for Continuous Monitoring (ID 23) }
	\label{img:treeid23}
\end{figure}

\begin{figure}[h]
	\centering
	\includegraphics[width=\textwidth]{figures/treeid24.png}
	\caption{J48 Decision Tree for Data-Driven Approach (ID 24)}
	\label{img:treeid24}
\end{figure}

\begin{figure}[h]
	\centering
	\includegraphics[width=\textwidth]{figures/treeid28.png}
	\caption{J48 Decision Tree for Statistical Pattern Recognition (ID 28)}
	\label{img:treeid28}
\end{figure}

\begin{figure}[h]
	\centering
	\includegraphics[width=\textwidth, height=\textheight]{figures/treeid36.png}
	\caption{J48 Decision Tree for Bayesian Model/Networks (ID 36)}
	\label{img:treeid36}
\end{figure}

\begin{figure}[h]
	\centering
	\includegraphics[width=\textwidth]{figures/treeid38.png}
	\caption{J48 Decision Tree for Artificial Intelligence Approach (ID 38)}
	\label{img:treeid38}
\end{figure}

\begin{figure}[h]
	\centering
	\includegraphics[width=\textwidth]{figures/treeid39.png}
	\caption{J48 Decision Tree for Artificial Neural Network (ID 39)}
	\label{img:treeid39}
\end{figure}

\begin{figure}[h]
	\centering
	\includegraphics[width=\textwidth]{figures/treeid40.png}
	\caption{J48 Decision Tree for Fuzzy Logic (ID 40)}
	\label{img:treeid40}
\end{figure}

\begin{figure}[h]
	\centering
	\includegraphics[width=\textwidth]{figures/treeid41.png}
	\caption{J48 Decision Tree for Model Approach (ID 41)}
	\label{img:treeid41}
\end{figure}

\begin{figure}[h]
	\centering
	\includegraphics[width=\textwidth]{figures/treeid49.png}
	\caption{J48 Decision Tree for No Prognostic Approach specified (ID 49)}
	\label{img:treeid49}
\end{figure}

\begin{figure}[h]
	\centering
	\includegraphics[width=\textwidth]{figures/treeid50.png}
	\caption{J48 Decision Tree for Degradation Process Modeling (ID 50)}
	\label{img:treeid50}
\end{figure}

\begin{figure}[h]
	\centering
	\includegraphics[width=\textwidth]{figures/treeid55.png}
	\caption{J48 Decision Tree for Root Cause Analysis (ID 55)}
	\label{img:treeid55}
\end{figure}

\begin{figure}[h]
	\centering
	\includegraphics[width=\textwidth]{figures/treeid56.png}
	\caption{J48 Decision Tree for Machinery Diagnostics (ID 56)}
	\label{img:treeid56}
\end{figure}

\begin{figure}[h]
	\centering
	\includegraphics[width=\textwidth]{figures/treeid57.png}
	\caption{J48 Decision Tree for No Fault Detection included (ID 57)}
	\label{img:treeid57}
\end{figure}

\begin{figure}[h]
	\centering
	\includegraphics[width=\textwidth]{figures/treeid58.png}
	\caption{J48 Decision Tree for Dynamic Action Scheduling (ID 58)}
	\label{img:treeid58}
\end{figure}

\begin{figure}[h]
	\centering
	\includegraphics[width=\textwidth]{figures/treeid59.png}
	\caption{J48 Decision Tree for (Auto.) Dynamic Spare Part Avail. (ID 59)}
	\label{img:treeid59}
\end{figure}

\begin{figure}[h]
	\centering
	\includegraphics[width=\textwidth]{figures/treeid60.png}
	\caption{J48 Decision Tree for No Scheduling included (ID 60)}
	\label{img:treeid60}
\end{figure}

\begin{figure}[h]
	\centering
	\includegraphics[width=\textwidth, height=\textheight]{figures/treeid61.png}
	\caption{J48 Decision Tree for Single-Component System (ID 61) }
	\label{img:treeid61}
\end{figure}

\begin{figure}[h]
	\centering
	\includegraphics[width=\textwidth]{figures/treeid62.png}
	\caption{J48 Decision Tree for Multi-Component System (ID 62)}
	\label{img:treeid62}
\end{figure}

\begin{figure}[h]
	\centering
	\includegraphics[width=\textwidth]{figures/treeid63.png}
	\caption{J48 Decision Tree for Economic Component Dependence (ID 63)}
	\label{img:treeid63}
\end{figure}

\begin{figure}[h]
	\centering
	\includegraphics[width=\textwidth]{figures/treeid64.png}
	\caption{J48 Decision Tree for Structural Component Dependence (ID 64)}
	\label{img:treeid64}
\end{figure}

\begin{figure}[h]
	\centering
	\includegraphics[width=\textwidth]{figures/treeid65.png}
	\caption{J48 Decision Tree for Stochastic Component Dependence (ID 65)}
	\label{img:treeid65}
\end{figure}

\begin{figure}[h]
	\centering
	\includegraphics[width=\textwidth]{figures/treeid66.png}
	\caption{J48 Decision Tree for Multi-Comp. Sys. w/o Dependencies (ID 66)}
	\label{img:treeid66}
\end{figure}

\begin{figure}[h]
	\centering
	\includegraphics[width=\textwidth]{figures/treeid69.png}
	\caption{J48 Decision Tree for Local Data Storage (ID 69)}
	\label{img:treeid69}
\end{figure}

\begin{figure}[h]
	\centering
	\includegraphics[width=\textwidth]{figures/treeid70.png}
	\caption{J48 Decision Tree for Remote/Cloud Data Storage (ID 70)}
	\label{img:treeid70}
\end{figure}

\begin{figure}[h]
	\centering
	\includegraphics[width=\textwidth]{figures/treeid71.png}
	\caption{J48 Decision Tree for Local Data Access (ID 71)}
	\label{img:treeid71}
\end{figure}

\begin{figure}[h]
	\centering
	\includegraphics[width=\textwidth]{figures/treeid72.png}
	\caption{J48 Decision Tree for Remote Data Access (ID 72)}
	\label{img:treeid72}
\end{figure}
